# Supplementary material for: A locally preferred structure characterises all dynamical regimes of a supercooled liquid
Source: arXiv:1502.01739 source file (2016-03-23)
Supplement: Supplementary file 1 [file Supplemental_Materials.pdf]

## Supplemental Materials

### 1. Methods: Classical Mechanics Simulations and Data Analysis

All molecular dynamics (MD) simulations were conducted using LAMMPS [22] using GPU-parallelization packages [S1]. Many-body atomic interactions in the  $\text{Cu}_{64}\text{Zr}_{36}$  system are described using the Finnis-Sinclair (FS) generalization of the embedded atom method (EAM) [23]. This semi empirical potential was selected for its ability to accurately reproduce the structures and properties of  $\text{Cu}_{64}\text{Zr}_{36}$  in both the liquid and glass regimes, as confirmed by comparisons made with both x-ray diffraction data and *ab initio* calculation results. The reported calorimetric glass formation temperature ( $T_g$ ) for this potential is approximately 750 K [23]. We confirm this by measuring the system volume, given zero average pressure, as a function of temperature, and identifying the temperature at which the thermal expansion coefficient changes (see Fig. 1).

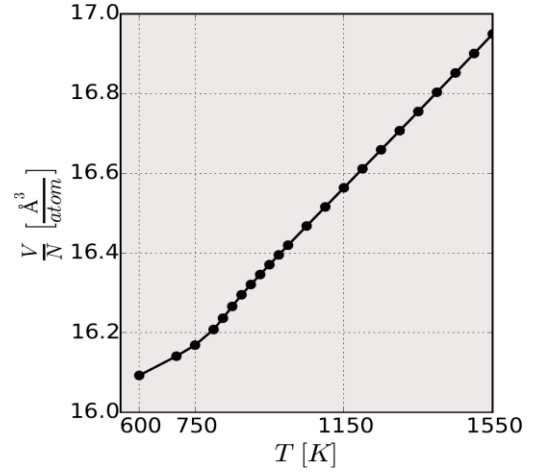

Figure 1. Volume per atom as a function of temperature. A change in the system's thermal expansion coefficient occurs near 750 K, which corresponds to  $T_g$ .

Simulations of constant  $N$ ,  $\langle P \rangle$ , and  $\langle T \rangle$  were conducted with  $\langle P \rangle = 0$ , using periodic boundary conditions, the Verlet integration method, and the Nose-Hoover thermostatting method. Each simulation was initialized with a random atomic configuration that evolves at  $T = 3300$  K for  $0.5$  ns to achieve equilibrium. The liquid was then quenched at a rate of  $10^{11} \frac{\text{K}}{\text{s}}$  down to its target temperature and subsequently relaxed for  $20$  ns before collecting structural and dynamical data. The integration timestep during the quenching and relaxation period was  $5$  fs. The integration step was then decreased to  $2$  fs and data was collected in snapshots at each time step. For a given target temperature, atomic-level data, such as the positions and velocities, were recorded for  $0.2$  ns; the system's Cauchy stress tensor (see below) was recorded for  $8$  ns. To ensure that the observed structural signatures represent the average, uncorrelated behavior of the system, an independent simulation of  $N = 30,000$  atoms was conducted for target temperature below  $T = 1000$  K as well as for  $1050$  K,  $2200$  K, and  $2500$  K. To check for system size effects, independent simulations of  $N = 10,000$  were also conducted for each temperature. The structure and local cluster times (discussed below) are assessed using a weighted-bisector Voronoi tessellation method [S2]. We performed Voronoi analysis on each system snap shot, comparing the structures between subsequent time steps. Voronoi cell faces comprising less than 0.5% of the cell's surface area were disregarded. The simulations of  $N = 30,000$  atoms were used to collect the Cauchy stress tensor and diffusivity data.

### 2. Local Structure Lifetimes, Chemical Ordering, and Dynamical Heterogeneity

There are two means that have been used interchangeably for measuring the lifetimes of local atomic configurations. Traditionally, both of these definitions consider an atom's nearest neighbors to be those that fall within a sphere of radius  $r_{min}$  centered on the atom. The hard cutoff,  $r_{min}$ , is taken to be the first minimum in the system's pair correlation function. First is the local cluster time (LCT), which is defined to be the average time required for an atom to lose or gain a nearest neighbor [14]. Second is the lifetime of local atomic connectivity (LLC) [S3]. For this measurement each atom is ascribed a unique ID, the IDs of the nearest neighbors of each atom is recorded at a time  $t = t_o$ . For  $t > t_o$ , the number of original nearest neighbors that persist for each atom is counted; the average number is recorded as  $N_c(t)$ . The LLC,  $\tau_{LC}$ , is thus defined to be the time required for the system, on average, to have locally lost one nearest neighbor:  $N_c(t_o + \tau_{LC}) = N_c(t_o) - 1$ .

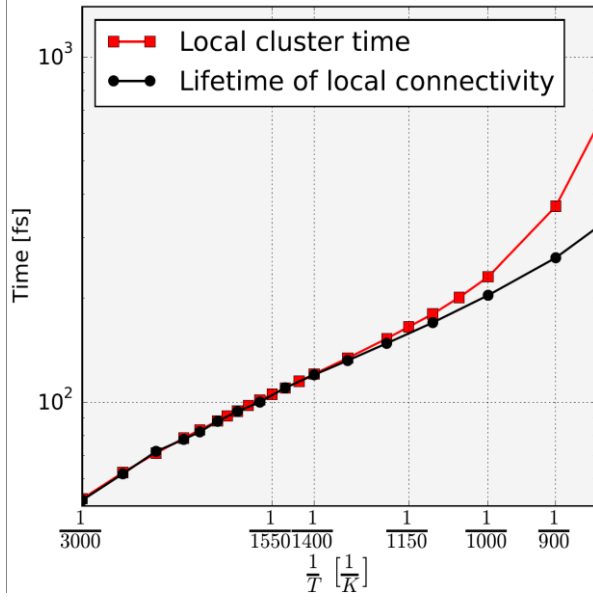

Figure 2. Comparison of the local cluster time (LCT) for Cu-centered clusters and the lifetime of the local connectivity (LLC).

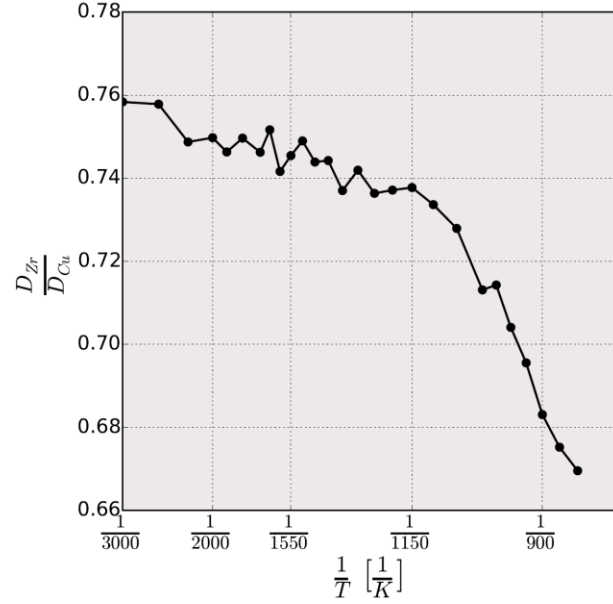

Figure 3. Ratio of the diffusivity of Zr atoms to the diffusivity of Cu atoms.

In our Letter, we utilize a weighted-bisector Voronoi tessellation method to analyze the local structures of our system and to determine an atom's nearest neighbors [S1]. Here, the nearest neighbors of an atom are defined to be its Voronoi neighbors. Though computationally intensive, this method is effectively temperature-sensitive, chemical species-sensitive, and is more meaningful from a structural perspective when determining an atom's structural environment than is using a hard-cutoff method. By comparing Voronoi analyses of consecutive simulation time steps, we are able to obtain accurate and precise measurements of the systems LCT and LLC.

Figure 2 shows, on a log scale, our measurements of the LCT for Cu-centered clusters and the system's LLC. Here we see that the two lifetimes are equal for temperatures above 1400 K. However, cooling below this temperature results in a significant enhancement of the LCT above the system's LLC. This growing disparity reflects the development of dynamical heterogeneities in the supercooled liquid. To understand this, consider that the system's LLC is sensitive to fast-changing local atomic structures, whereas the LCT treats fast and slow-changing structures on an equal footing. For example, in the time required for a stable cluster to lose one of its atoms, an unstable configuration may have lost three atoms. Therefore, the value of  $N_c(t)$  will decrease as the fast-changing structures lose multiple constituents and will thus yield a short LLC. The LCT, on the other hand, reflects the time needed for an average cluster to lose a single atom, and is enhanced by the presence of long-lived clusters. Posed another way, the LLC is more a measure of diffusion in the system, and thus is controlled by fast-changing structures, whereas LCT is a measure of its structural relaxation. The result shown in Figure 2 demonstrates the coexistence of regions of stable atomic configurations along with highly active ones, which grow in extent and dynamical disparity as the system is cooled towards  $T_g$ .

We now consider the supercooled liquid's dynamical heterogeneity in the context of its frustration-limited domains (FLDs) of connected icosahedra and the chemical ordering that they exhibit. The Cu-centered icosahedra that form in  $\text{Cu}_{64}\text{Zr}_{36}$  prefer a packed structure that is Zr-rich in comparison to the alloy's composition. Across a broad range of temperatures, the average composition of the 13-atom icosahedron is approximately  $\text{Cu}_{57}\text{Zr}_{43}$  [30]. Once FLDs comprise a significant portion of the liquid's structure, icosahedra preserve their preferred Zr-rich local environment in a Zr-poor alloy by sharing Zr atoms with one another. The vertex, edge, and face connections preferentially incorporate Zr atoms in comparison to the icosahedron-shell composition, with over 75% of the vertex connections consisting of a Zr atom [30]. In terms of dynamics, the role that Zr plays in facilitating

connections amongst icosahedra impacts its diffusivity. Figure 3 demonstrates this by plotting the ratio of the diffusivities of Zr to Cu. Below  $T_D$  (1150 K), FLDs exhibit rapid growth and correspondingly the diffusivity of Zr drops quickly. The system's atomic motions thus begin to decouple as Zr atoms are incorporated into the stable domains of icosahedra, which exist amidst dynamically active Cu-rich regions of the supercooled liquid [30,37]. This provides a clear structural perspective of the separation of timescales shown in Figure 2 and links the development of dynamical heterogeneity with structural ordering in the liquid.

### 3. Two-Step Relaxation and Diffusivities

To detail the development of heterogeneous, glassy dynamics of supercooled  $\text{Cu}_{64}\text{Zr}_{36}$  in the context of a characteristic two-step relaxation process, we measured the tagged-particle time-dependent mean square displacement (MSD) across a broad temperature range. The results are shown in Figure 4 for temperatures ranging from 2000 K to 800 K in 100 K intervals. At high temperatures, particles simply undergo short-time ballistic motion before entering the asymptotic long-time diffusive regime. On a log-log plot, the y-intercept of the long-time asymptote is proportional to the particle's diffusivity [4]. The temperature dependence of these diffusivities are provided in the main text of the Letter. A small downward shift is observed with decreasing temperature in the short-time portions of the curves - this is simply caused by the kinetic reduction in the particle's mean speed. The accelerating drop in diffusivity, on the other hand, reflects the development of a sustained plateau in time that separates fast and slow relaxation processes in the supercooled liquid [3,4]. Tracking the temperature dependence of the particle diffusivities thus provides a means for identifying the approximate temperature where the system begins to exhibit non-exponential relaxations in its dynamic correlation functions. As concluded in the Letter, a plateau begins to develop as the liquid is cooled below  $T_D$  (1050 K), marking the gradual onset of so-called glassy dynamics in the system.

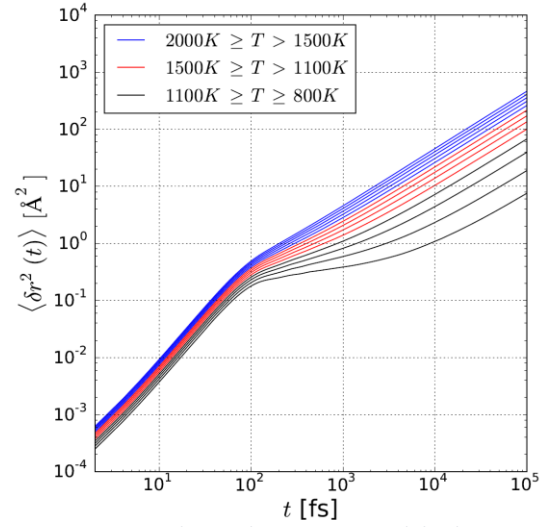

Figure 4. Tagged-particle mean squared displacement as a function of time on a log-log scale. The consecutive temperatures presented are separated by  $\Delta T = 100$  K steps.

### 4. Viscosity and the Cauchy Stress Tensor

The liquid viscosity was calculated using the Green-Kubo formula:

$$\eta = \frac{V}{k_B T} \int_0^\infty \langle \sigma_{ij}(t) \sigma_{ij}(0) \rangle dt$$

where  $V$  is the system volume,  $T$  is the temperature,  $k_B$  is the Boltzmann constant, and  $\sigma_{ij}(t)$  is an off-diagonal element of the time-dependent Cauchy stress tensor. The stress tensor can be calculated from summing atomic-quantities:

$$\sigma_{ij} = \frac{1}{V} \sum_{\alpha} \left( m^{\alpha} \vec{v}_i^{\alpha} \vec{v}_j^{\alpha} + \sum_{\beta > \alpha} \vec{F}_i^{\alpha\beta} (\vec{r}^{\alpha} - \vec{r}^{\beta})_j \right)$$

where  $m$ ,  $\vec{v}$ , and  $\vec{r}$  are the mass, velocity, and position of a particle.  $\alpha$  and  $\beta$  are summation indices that run over each atom.  $i, j$  are cartesian component indices.  $\vec{F}^{\alpha\beta}$  is the force exerted on particle  $\alpha$  due to particle  $\beta$ .

## References

- [S1] W.M Brown and Y. Masako. Comp Phys Comm **184**, 2785-2793 (2013)
- [S2] J. Park and Y. Shibutani. Intermetallics **15**, 187-192 (2007).
- [S3] T. Iwashita and T. Egami. Phys Rev Lett **108**, 196001 (2012)
